# Supplementary material for: Shallow and Deep Convolutional Networks for Saliency Prediction
Source: arXiv:1603.00845 source file (2016-03-02)
Supplement: Supplementary file 1 [file 7_additional.tex]

\section{Additional material}

Table \ref{tab:light} contains the details for the memory requirements of the light network. As in most ConvNets, the highest memory requirements correspond to the early convolutional layers, while the largest amount of parameters are associated to the fully connected layers at the deepest level of the network.

\begin{table*}
\begin{center}
\begin{tabular}{|l|c|c|}
\hline
Layer		& 	Blob Data Size			 & Filter Weights   \\
			& 	[Width x Height x Depth] & [( convX x convY x DepthIn ) x Depth]    \\
\hline
input 		& 96x96x3 = 27,648			& 0 \\
conv5-32 	& 92x92x32	= 270,848 		& (5x5x3)x32+32= 2,400\\
maxpool2 	& 46x46x32 	= 67,712		& 0 \\
conv3-64 	& 44x44x64  = 123,904		& (3x3x32)x64+64= 18,496\\
maxpool2 	& 22x22x64  = 30,976		& 0 \\
conv3-128 	& 20x20x128  = 30,976		& (3x3x64)x128+128= 73,856 \\
maxpool2 	& 10x10x128  = 12,800		& 0 \\
FC-4608 	& 1x1x4608  = 4,608			& (1x1x12,800)x4,608+4,608= 58,987,008\\
slice1 		& 1x1x2304  = 2,304			& 0 \\
slice2 		& 1x1x2304  = 2,304			& 0 \\
maxout 		& 1x1x2304  = 2,304			& 0 \\
FC-2304 	& 1x1x2304  = 2,304			& (1x1x2,304)x2,304+2,304= 5,310,720\\
output		& 1x48x48 = 2,304			&   \\
\hline
Total 		& 601,216					& 64,392,512 \\
Memory (train) 	& 4.58 MB				& - \\
Memory (test) 	& 2.29 MB 				& 246 MB \\
\hline
\end{tabular}
\end{center}
\caption{Memory requirements for the proposed shallow ConvNet.}
\label{tab:light}
\end{table*}
